# Supplementary material for: A Family of Distributions of Random Subsets for Controlling Positive and Negative Dependence
Source: arXiv:2408.01022 source file (2025-02-10)
Supplement: Supplementary file 1 [file supplement.tex]

\documentclass[twoside]{article}

\usepackage{aistats2025}

% If you use natbib package, activate the following three lines:
\usepackage[round]{natbib}

% If you use BibTeX in apalike style, activate the following line:
%\bibliographystyle{apalike}

%%% packages
\usepackage{amsmath, amssymb, amsthm}
\usepackage{bm, bbm}
\usepackage{mathtools}
\usepackage{hyperref}
\usepackage{xcolor}
\usepackage{subcaption}
\usepackage[group-minimum-digits = 4, group-separator = {,}]{siunitx}

\usepackage{xr}

%%% Theorems
\theoremstyle{plain}

\theoremstyle{definition}

\theoremstyle{remark}

%%% Symbols
\newcommand*{\tr}{\mathrm{tr}}

% If your paper is accepted, change the options for the package
% aistats2025 as follows:
%
%\usepackage[accepted]{aistats2025}
%
% This option will print headings for the title of your paper and
% headings for the authors names, plus a copyright note at the end of
% the first column of the first page.

% If you set papersize explicitly, activate the following three lines:
%\special{papersize = 8.5in, 11in}
%\setlength{\pdfpageheight}{11in}
%\setlength{\pdfpagewidth}{8.5in}

% If you use natbib package, activate the following three lines:
%\usepackage[round]{natbib}
%\renewcommand{\bibname}{References}
%\renewcommand{\bibsection}{\subsubsection*{\bibname}}

% If you use BibTeX in apalike style, activate the following line:
%\bibliographystyle{apalike}

\begin{document}

% If your paper is accepted and the title of your paper is very long,
% the style will print as headings an error message. Use the following
% command to supply a shorter title of your paper so that it can be
% used as headings.
%
%\runningtitle{I use this title instead because the last one was very long}

% If your paper is accepted and the number of authors is large, the
% style will print as headings an error message. Use the following
% command to supply a shorter version of the authors names so that
% they can be used as headings (for example, use only the surnames)
%
%\runningauthor{Surname 1, Surname 2, Surname 3, ...., Surname n}

% Supplementary material: To improve readability, you must use a single-column format for the supplementary material.
\onecolumn
\aistatstitle{Instructions for Paper Submissions to AISTATS 2025: \\
Supplementary Materials}

\renewcommand{\theequation}{\thesection.\arabic{equation}}
\setcounter{equation}{0}

\section{Proofs}\label{app:proofs}
\subsection{Proof of Proposition \ref{prop:dkpp_bm}}
\begin{proof}
    Let $\mathcal{A} \subseteq \mathcal{Y}$ be a random subset following the DKPP $P_\phi(\mathcal{A}; \bm{L})$,
    and let $\bm{z} = (z_1, \ldots, z_N)^\top$ denote the indicator vector of $\mathcal{A}$:
    \begin{align}
        z_i =
        \left \{~
        \begin{aligned}
            0 & \quad\mbox{if}~ i \notin \mathcal{A},\\
            1 & \quad\mbox{if}~ i \in \mathcal{A},\\
        \end{aligned}
        \right .
    \end{align}
    for $i = 1, \ldots, N$.
    Then, we obtain
    \begingroup
    \allowdisplaybreaks
    \begin{align}
        P_\phi(\mathcal{A}; \bm{L}) &\propto \exp \tr \phi(\bm{L}[\mathcal{A}])\\
        &= \exp \tr \left ( a \bm{L}[\mathcal{A}]\bm{L}[\mathcal{A}]  + b \bm{L}[\mathcal{A}] + c\bm{I} \right )\\
        &= \exp \left ( a \tr \bm{L}[\mathcal{A}]\bm{L}[\mathcal{A}] + b \tr \bm{L}[\mathcal{A}] + c \lvert \mathcal{A} \rvert \right )\\
        &= \exp \left ( a \lVert \bm{L}[\mathcal{A}] \rVert^2_F + b \tr \bm{L}[\mathcal{A}] + c \lvert \mathcal{A} \rvert \right )\\
        &= \exp \left ( a \sum_{i,j \in \mathcal{A}} \lvert L_{ij} \rvert^2 + \sum_{i \in \mathcal{A}} (b L_{ii} + c) \right )\\
        &= \exp \left ( a \sum^N_{i,j = 1} \lvert L_{ij} \rvert^2 z_i z_j + \sum^N_{i = 1} (b L_{ii} + c) z_i \right )\\
        &= \exp \left ( a \sum_{i \neq j} \lvert L_{ij} \rvert^2 z_i z_j + a\sum^N_{i=1} L^2_{ii} z^2_i + \sum^N_{i = 1} (b L_{ii} + c) z_i \right )\\
        &= \exp \left ( a \sum_{i \neq j} \lvert L_{ij} \rvert^2 z_i z_j + a\sum^N_{i=1} L^2_{ii} z_i + \sum^N_{i = 1} (b L_{ii} + c) z_i  \right )\\
        \label{eq:proof1}
        &= \exp \left ( a \sum_{i \neq j} \lvert L_{ij} \rvert^2 z_i z_j + \sum^N_{i=1} (a L^2_{ii} + b L_{ii} + c) z_i \right ).
    \end{align}
    \endgroup
    By comparing \eqref{eq:proof1} and \eqref{eq:boltzmann_machine}, we prove the proposition.
\end{proof}

\subsection{Proof of Proposition \ref{prop:affine_logmod}}
\begin{proof}
    \ \\
    \textsf{[$\phi$ is affine$~\Longrightarrow~$DKPP is log-modular]}\par
    We denote the diagonal matrix with the eigenvalues of $\bm{L}[\mathcal{A}]$ by $\bm{\Lambda}_\mathcal{A}$.
    By letting $\phi(x) = bx + c$ from the assumption, we find that the log-likelihood of the DKPP is
    \begin{align}
        \log P_\phi(\mathcal{A}; \bm{L}) = \tr\phi(\bm{L}[\mathcal{A}]) - \log Z_\phi(\bm{L})
        &= \tr(b \bm{\Lambda}_\mathcal{A} + c\bm{I}) - \log Z_\phi(\bm{L})\\
        &= b \tr\bm{\Lambda}_\mathcal{A} + c \lvert \mathcal{A} \rvert - \log Z_\phi(\bm{L})\\
        &= b \tr\bm{L}_\mathcal{A} + c \lvert \mathcal{A} \rvert - \log Z_\phi(\bm{L})\\
        \label{eq:dkpp_linear_loglikelihood}
        &= \sum_{i \in \mathcal{A}} (b L_{ii} + c) - \log Z_\phi(\bm{L}).
    \end{align}
    This is a modular function for $\mathcal{A} \subseteq \mathcal{Y}$.
    
    \textsf{[DKPP is log-modular $~\Longrightarrow~$ $\phi$ is affine]}\par
    From the log-modularity of the DKPP, we have
    \begin{align}
        \label{eq:dkpp_logmodularity}
        \tr\phi(\bm{L}[\mathcal{S}]) + \tr\phi(\bm{L}[\mathcal{T}])
        = \tr\phi(\bm{L}[\mathcal{S} \cup \mathcal{T}]) + \tr\phi(\bm{L}[\mathcal{S} \cap \mathcal{T}])
    \end{align}
    for every $\mathcal{S}, \mathcal{T} \subseteq \mathcal{Y}$.
    %By defining some nonlinear $g: \mathbb{R} \to \mathbb{R}$ such that $g(0) = 0$,
    By defining $g(x) \coloneqq \phi(x) - \phi(0)$,
    we can represent $\phi$ as $\phi(x) = g(x) + \phi(0)$.
    Now, we take $\mathcal{S} = \{i\}, \mathcal{T} = \{j\}~ (i \neq j)$ and
    the kernel matrix $\bm{L}$ arbitrarily to satisfy $L_{ij} = \sqrt{L_{ii} L_{jj}} \in \mathbb{R}$.
    Since $\bm{L}$ and $\phi$ are independent, this choice of $\bm{L}$ does not impose any restriction on $\phi$.
    
    The two eigenvalues of $\bm{L}[\mathcal{S} \cup \mathcal{T}] \in \mathbb{R}^{2 \times 2}$ are given by $\lambda_1 = L_{ii} + L_{jj}$ and $\lambda_2 = 0$.
    The l.h.s. of \eqref{eq:dkpp_logmodularity} is
    \begin{align}
        \label{eq:logmodular_linear_lhs}
        \tr\phi(\bm{L}[\mathcal{S}]) + \tr\phi(\bm{L}[\mathcal{T}])
        = \phi(L_{ii}) + \phi(L_{jj}),
    \end{align}
    and the r.h.s. is
    \begin{align}
        \tr\phi(\bm{L}[\mathcal{S} \cup \mathcal{T}]) + \tr\phi(\bm{L}[\mathcal{S} \cap \mathcal{T}])
        = \tr\phi(\bm{L}[\mathcal{S} \cup \mathcal{T}])
        = \phi(\lambda_1) + \phi(\lambda_2).
    \end{align}
    Therefore, we have the identity
    \begin{align}
        \label{eq:logmodular_linear}
        \phi(L_{ii}) + \phi(L_{jj})
        = \phi(\lambda_1) + \phi(\lambda_2).
    \end{align}
    By substituting $\phi(x) = g(x) + \phi(0)$ into \eqref{eq:logmodular_linear}, it becomes
    \begin{align}
        & \{g(L_{ii}) + \phi(0)\} + \{g(L_{jj}) + \phi(0)\}
        = \{g(\lambda_1) + \phi(0)\} + \{g(\lambda_2) + \phi(0)\}\\
        &\quad \Longleftrightarrow~ g(L_{ii}) + g(L_{jj}) = g(\lambda_1) + g(\lambda_2) = g(L_{ii} + L_{jj}) + g(0) = g(L_{ii} + L_{jj}).
    \end{align}
    This means that $g$ must be linear and $\phi$ must be affine.
\end{proof}

\subsection{Proof of Proposition \ref{prop:marginal_rao_blackwell}}
\begin{proof}
We consider the partition of $\mathcal{Y}$ given by
$\mathcal{A}_{\mathrm{in}}, \mathcal{Y} \backslash \mathcal{A}_{\mathrm{out}}, \mathcal{A}_{\mathrm{out}} \backslash \mathcal{A}_{\mathrm{in}}$
and
separate the random vector $\bm{\xi} = (\xi_1, \ldots, \xi_N)^\top$ by
$
\bm{\xi}^+ \coloneqq (\xi_i)_{i \in \mathcal{A}_{\mathrm{in}}},
\bm{\xi}^- \coloneqq (\xi_i)_{i \in \mathcal{Y} \backslash \mathcal{A}_{\mathrm{out}}}
$, and
$\bm{\xi}^\circ \coloneqq (\xi_i)_{i \in \mathcal{A}_{\mathrm{out}} \backslash \mathcal{A}_{\mathrm{in}}}$.
For example, when
$\mathcal{Y} = \{1, 2, 3, 4, 5\}, \mathcal{A}_{\mathrm{in}} = \{1, 2\}$,
and $\mathcal{A}_{\mathrm{out}} = \{1, 2, 4, 5\} (\supseteq \mathcal{A}_{\mathrm{in}})$,
the separation of $\bm{\xi}$ becomes
$\bm{\xi}^+ = (\xi_1, \xi_2)^\top, \bm{\xi}^- = (\xi_3)$, and $\bm{\xi}^\circ = (\xi_4, \xi_5)^\top$.
We also denote
$N^+ \coloneqq \lvert \mathcal{A}_{\mathrm{in}} \rvert,~
N^- \coloneqq \lvert \mathcal{Y} \backslash \mathcal{A}_{\mathrm{out}} \rvert$,
and
$N^\circ \coloneqq \lvert \mathcal{A}_{\mathrm{out}} \backslash \mathcal{A}_{\mathrm{in}} \rvert$
and
$\bm{\xi}^+ \sim Q_{\bm{q}^+},\bm{\xi}^- \sim Q_{\bm{q}^-}$,
and $\bm{\xi}^\circ \sim Q_{\bm{q}^\circ}$,
where
$Q_{\bm{q}^+} \coloneqq \prod_{i \in \mathcal{A}_{\mathrm{in}}} Q_{q_i}(\xi_i),
Q_{\bm{q}^-} \coloneqq \prod_{i \in \mathcal{Y} \backslash \mathcal{A}_{\mathrm{out}}} Q_{q_i}(\xi_i)$,
and 
$Q_{\bm{q}^\circ} \coloneqq \prod_{i \in \mathcal{A}_{\mathrm{out}} \backslash \mathcal{A}_{\mathrm{in}}} Q_{q_i}(\xi_i)$.
We denote the probability measure that induces $Q_{\bm{q}^+}$ by $\mathbb{Q}_{\bm{q}^+}$ and the same for $\mathbb{Q}_{\bm{q}^-}$ and $\mathbb{Q}_{\bm{q}^\circ}$.

As shown in \eqref{eq:marginal_is}, 
$
    \mathbb{E}_{\bm{\xi} \sim Q_{\bm{q}}}[w(\mathcal{A}_{\bm{\xi}}) \mathbbm{1} (\mathcal{A}_{\mathrm{in}} \subseteq \mathcal{A}_{\bm{\xi}} \subseteq \mathcal{A}_{\mathrm{out}})]
$
is equal to
$\mathbb{P}(\mathcal{A}_{\mathrm{in}} \subseteq \mathcal{A} \subseteq \mathcal{A}_{\mathrm{out}})$.
The tower property of expectation states that
$\mathbb{E}_X[f(X)] = \mathbb{E}_Y [\mathbb{E}_X [f(X) \vert Y]]$ generally holds
for an arbitrary pair of random variables $(X, Y)$ and an arbitrary function $f$.
By choosing $X \gets \bm{\xi}$ and
$Y \gets \bm{\xi}^+$ (and $Y \gets \bm{\xi}^-$), we have
\begin{align}
    \mathbb{P}(\mathcal{A}_{\mathrm{in}} \subseteq \mathcal{A} \subseteq \mathcal{A}_{\mathrm{out}})
    &= \mathbb{E}_{\bm{\xi} \sim Q_{\bm{q}}}[w(\mathcal{A}_{\bm{\xi}})
    \mathbbm{1} (\mathcal{A}_{\mathrm{in}} \subseteq \mathcal{A}_{\bm{\xi}} \subseteq
    \mathcal{A}_{\mathrm{out}})]\\
    &= \mathbb{E}_{\bm{\xi}^+}[\mathbb{E}_{\bm{\xi}^-, \bm{\xi}^\circ}[w(\mathcal{A}_{\bm{\xi}})
    \mathbbm{1} (\mathcal{A}_{\mathrm{in}} \subseteq \mathcal{A}_{\bm{\xi}} \subseteq
    \mathcal{A}_{\mathrm{out}}) \vert \bm{\xi}^+]]\\
    &= \sum_{z_1 \in \{0, 1\}} \cdots \sum_{z_{N^+} \in \{0, 1\}}
    \mathbb{Q}_{\bm{q}^+}(\xi^+_1 = z_1, \ldots, \xi^+_{N^+} = z_{N^+})\\
    &\hphantom{
        \sum_{z_1 \in \{0, 1\}} \cdots \sum_{z_{N^+} \in \{0, 1\}}
    }
    \times\mathbb{E}_{\bm{\xi}^-, \bm{\xi}^\circ}[w(\mathcal{A}_{\bm{\xi}})
    \underbrace{
    \mathbbm{1} (\mathcal{A}_{\mathrm{in}} \subseteq \mathcal{A}_{\bm{\xi}} \subseteq
    \mathcal{A}_{\mathrm{out}})}_{\mathclap{\mbox{{\footnotesize takes $0$ if not $\xi^+_1 = \cdots =  \xi^+_{N^+} = 1$}}}}
    \vert \bm{\xi}^+ = \bm{z}]\\
    &= \mathbb{Q}_{\bm{q}^+}(\xi^+_1 = 1, \ldots, \xi^+_{N^+} = 1)
    \mathbb{E}_{\bm{\xi}^-, \bm{\xi}^\circ}[w(\mathcal{A}_{\bm{\xi}})
    \mathbbm{1} (\mathcal{A}_{\mathrm{in}} \subseteq \mathcal{A}_{\bm{\xi}} \subseteq
    \mathcal{A}_{\mathrm{out}}) \vert \bm{\xi}^+ = \bm{1}]\\
    &= Q_{\bm{q}^+}(\bm{1})
    \mathbb{E}_{\bm{\xi}^-}[
    \mathbb{E}_{\bm{\xi}^\circ}[w(\mathcal{A}_{\bm{\xi}})
    \mathbbm{1} (\mathcal{A}_{\mathrm{in}} \subseteq \mathcal{A}_{\bm{\xi}} \subseteq
    \mathcal{A}_{\mathrm{out}}) \vert \bm{\xi}^+ = \bm{1}, \bm{\xi}^-]]\\
    &= Q_{\bm{q}^+}(\bm{1})
    \sum_{z_1 \in \{0, 1\}} \cdots \sum_{z_{N^-} \in \{0, 1\}}
    \mathbb{Q}_{\bm{q}^-}(\xi^-_1 = z_1, \ldots, \xi^-_{N^-} = z_{N^-})\\
    &\hphantom{
        = Q_{\bm{q}^+}(\bm{1})
        \sum_{z_1 \in \{0, 1\}} \cdots \sum_{z_{N^-} \in \{0, 1\}}
    }\times
    \mathbb{E}_{\bm{\xi}^\circ}[w(\mathcal{A}_{\bm{\xi}})
    \underbrace{
    \mathbbm{1} (\mathcal{A}_{\mathrm{in}} \subseteq \mathcal{A}_{\bm{\xi}} \subseteq
    \mathcal{A}_{\mathrm{out}})}_{\mathclap{\mbox{{\footnotesize takes $0$ if not $\xi^-_1 = \cdots = \xi^-_{N^+} = 0$}}}}
    \vert \bm{\xi}^+ = \bm{1}, \bm{\xi}^- = \bm{z}]\\
    &=Q_{\bm{q}^+}(\bm{1}) Q_{\bm{q}^-}(\bm{0})
    \mathbb{E}_{\bm{\xi}^\circ}[w(\mathcal{A}_{\bm{\xi}})
    \mathbbm{1} (\mathcal{A}_{\mathrm{in}} \subseteq \mathcal{A}_{\bm{\xi}} \subseteq
    \mathcal{A}_{\mathrm{out}})
    \vert \bm{\xi}^+ = \bm{1}, \bm{\xi}^- = \bm{0}]\\
    &=Q_{\bm{q}^+}(\bm{1}) Q_{\bm{q}^-}(\bm{0})
    \mathbb{E}_{\bm{\xi}^\circ}[w(\mathcal{A}_{\bm{\xi}})
    \vert \bm{\xi}^+ = \bm{1}, \bm{\xi}^- = \bm{0}]\\
    &=Q_{\bm{q}^+}(\bm{1}) Q_{\bm{q}^-}(\bm{0})
    \mathbb{E}_{\bm{\xi}^\circ} \left [ \left .
    \frac{P(\mathcal{A}_{\bm{\xi}})}{Q_{\bm{q}}(\bm{\xi})}
    \right \vert \bm{\xi}^+ = \bm{1}, \bm{\xi}^- = \bm{0} \right ]\\
    &= \mathbb{E}_{\bm{\xi}^\circ} \left [ \left .
    \frac{P(\mathcal{A}_{\bm{\xi}})}{Q_{\bm{q}^\circ}(\bm{\xi}^\circ)}
    \right \vert \bm{\xi}^+ = \bm{1}, \bm{\xi}^- = \bm{0} \right ],
\end{align}
which is the first half of Proposition \ref{prop:marginal_rao_blackwell}.

On the other hand, the tower property of variance states that
$
\mathrm{Var}_X[f(X)] = \mathbb{E}_Y[\mathrm{Var}_X[f(X) \vert Y]] + \mathrm{Var}_Y[\mathbb{E}_X[f(X) \vert Y]]
\leq \mathrm{Var}_Y[\mathbb{E}_X[f(X) \vert Y]].
$
This ensures the latter half of Proposition \ref{prop:marginal_rao_blackwell}.
\end{proof}

\subsection{Proof of Proposition \ref{prop:marginal_cardinality}}
\begin{proof}
    First, we define independent Bernoulli trials
    $Q_{\bm{q}}$ as in \eqref{eq:variational_distribution}
    with $q_1 = \cdots = q_N \eqqcolon q$.
    By importance sampling, we have
    \begin{align}
        \mathbb{P}(\lvert \mathcal{A} \rvert = k)
        = \sum_{\mathcal{A}: \lvert \mathcal{A} \rvert = k} P (\mathcal{A})
        = \mathbb{E}_{\mathcal{A} \sim P}[\mathbbm{1} (\lvert \mathcal{A} \rvert = k)]
        \label{eq:marginal_ls_cardinality_1}
        = \mathbb{E}_{\bm{\xi} \sim Q_{\bm{q}}}[w(\mathcal{A}_{\bm{\xi}}) \mathbbm{1} (\lvert \mathcal{A}_{\bm{\xi}} \rvert = k)]
    \end{align}
    in the similar way to \eqref{eq:marginal_is},
    where $w(\mathcal{A}_{\bm{\xi}}) = P(\mathcal{A}_{\bm{\xi}}) / Q_{\bm{q}}(\bm{\xi})$
    is the weight function.
    Then, we introduce a new random variable,
    $\zeta \coloneqq \sum^N_{i=1} \xi_i$,
    that follows the binomial distribution: $\xi \sim \mathrm{Bin}(N, q)$.
    Now, we consider the Rao--Blackwellization of \eqref{eq:marginal_ls_cardinality_1} by the auxiliary random variable $\zeta$:
    \begin{align}
        \mathbb{P}(\lvert \mathcal{A} \rvert = k)
        &= \mathbb{E}_{\bm{\xi}}[w(\mathcal{A}_{\bm{\xi}}) \mathbbm{1} (\lvert \mathcal{A}_{\bm{\xi}} \rvert = k)]\\
        &= \mathbb{E}_{\zeta} \left [\mathbb{E}_{\bm{\xi}} \left [w(\mathcal{A}_{\bm{\xi}}) \mathbbm{1} (\lvert \mathcal{A}_{\bm{\xi}} \rvert = k) \left \vert \sum^N_{i=1} \xi_i = \zeta \right . \right ] \right ]\\
        &= \sum^N_{n = 0} \mathbb{P}(\zeta = n) \mathbb{E}_{\bm{\xi}} \left [ w(\mathcal{A}_{\bm{\xi}}) 
        \underbrace{\mathbbm{1} (\lvert \mathcal{A}_{\bm{\xi}} \rvert = k)}_{\mathclap{\mbox{{\footnotesize takes 0 if $\zeta \neq k$}}}}
        \left \vert \sum^N_{i=1} \xi_i = n \right . \right ]\\
        &= \mathbb{P}(\zeta = k) \mathbb{E}_{\bm{\xi}}\left [w(\mathcal{A}_{\bm{\xi}}) \left \vert \sum^N_{i=1} \xi_i = k \right . \right ]\\
        &= \binom{N}{k} q^{k} (1-q)^{N-k} \mathbb{E}_{\bm{\xi}} \left [ \frac{P(\mathcal{A}_{\bm{\xi}})}{Q_{\bm{q}}(\mathcal{A}_{\bm{\xi}})} \left \vert \sum^N_{i=1} \xi_i = k \right .\right ]\\
        &= \binom{N}{k} q^{k} (1-q)^{N-k} \mathbb{E}_{\bm{\xi}} \left [ \frac{P(\mathcal{A}_{\bm{\xi}})}{q^k (1-q)^{N-k}} \left \vert \sum^N_{i=1} \xi_i = k \right .\right ]\\
        \label{eq:marginal_ls_cardinality}
        &= \binom{N}{k} \mathbb{E}_{\bm{\xi}} \left [ P(\mathcal{A}_{\bm{\xi}}) \left \vert \sum^N_{i=1} \xi_i = k \right . \right ].
    \end{align}
    Because $\xi_1, \ldots, \xi_N$ are i.i.d. such that $\xi_i \sim \mathrm{Bernoulli}(q)$,
    the conditional expectation in the r.h.s. of \eqref{eq:marginal_ls_cardinality}
    equals to the expectation over the uniform distribution on $\{\mathcal{A} \subseteq \mathcal{Y} : \lvert \mathcal{A} \rvert = k\}$.
\end{proof}

\section{Mean-field Approximation}\label{app:mean_field}
We derive the update rule of the mean-field approximation \eqref{eq:mean_field_update} for completeness.
It is recommended to also refer to the thesis by \citet[Section 3]{djolonga2018} since the derivation is equivalent.
Let $\bm{\xi} \in \{0, 1\}^N$ denote a binary random vector,
$f: 2^\mathcal{Y} \to \mathbb{R}$ be a set function,
and $P: \bm{\xi} \mapsto Z^{-1} \exp (f(\mathcal{A}_{\bm{\xi}}))$ be a probabilistic function on $\{0, 1\}^N$, or equivalently $2^\mathcal{Y}$.
Now, we consider minimizing $\mathrm{KL}(Q_{\bm{q}} \Vert P)$, where $Q_{\bm{q}}$ is defined in \eqref{eq:variational_distribution}.
Given
\begin{align}
    \mathrm{KL}(Q_{\bm{q}} \Vert P)
    = \mathbb{E}_{\bm{\xi} \sim Q_{\bm{q}}}\left [ \log \frac{Q_{\bm{q}} (\bm{\xi})}{P(\bm{\xi})} \right ]
    = \mathbb{E}_{\bm{\xi} \sim Q_{\bm{q}}} [ \log Q_{\bm{q}} (\bm{\xi}) ]
    - \mathbb{E}_{\bm{\xi} \sim Q_{\bm{q}}}[ f(\mathcal{A}_{\bm{\xi}}) ] + \log Z,
\end{align}
the minimization of $\mathrm{KL}(Q_{\bm{q}} \Vert P)$ is equivalent to maximizing the ELBO,
defined as
\begin{align}
    L(\bm{q}) \coloneqq
    -\mathbb{E}_{\bm{\xi} \sim Q_{\bm{q}}} [ \log Q_{\bm{q}} (\bm{\xi}) ]
    + \mathbb{E}_{\bm{\xi} \sim Q_{\bm{q}}}[ f(\mathcal{A}_{\bm{\xi}}) ]
    ~(= \mathbb{H}[Q_{\bm{q}}] + \tilde{f}(\bm{q})).
\end{align}
We solve the problem $\max_{\bm{q}} L(\bm{q})$ by using the coordinate ascent.
The derivative $\frac{\partial L(\bm{q})}{\partial q_i}$ is 
\begin{align}
    \frac{\partial L(\bm{q})}{\partial q_i}
    &= \frac{\partial L(\bm{q})}{\partial q_i}
    \left \{
    \sum^N_{j=1} (-q_j \log q_j - (1 - q_j) \log (1 - q_j))
    + \sum_{\mathcal{A} \subseteq \mathcal{Y}} f(\mathcal{A}) \prod_{j \in \mathcal{A}} q_j \prod_{j \notin \mathcal{A}} (1 - q_j)
    \right \}\\
    &= \log \frac{1-q_i}{q_i}
    + \sum_{\mathcal{A}: i \in \mathcal{A}} f(\mathcal{A}) \prod_{\substack{j \in \mathcal{A}\\j \neq i}} q_j \prod_{j \notin \mathcal{A}} (1 - q_j)
    - \sum_{\mathcal{A}: i \notin \mathcal{A}} f(\mathcal{A}) \prod_{j \in \mathcal{A}} q_j \prod_{\substack{j \notin \mathcal{A} \\ j \neq i}} (1 - q_j)\\
    &= \log \frac{1-q_i}{q_i}
    + \sum_{\mathcal{A} \subseteq \mathcal{Y} \backslash \{i\}} [f(\mathcal{A} \cup \{i\}) - f(\mathcal{A})]
    \prod_{j \in \mathcal{A}} q_j \prod_{j \notin \mathcal{A}} (1 - q_j)\\
    &= \log \frac{1-q_i}{q_i} + \mathbb{E}_{\bm{\xi}_{\backslash i} \sim Q_{\bm{q}_{\backslash i}}} [f(i \vert \mathcal{A}_{\bm{\xi}_{\backslash i}})].
\end{align}
By solving the equation
\begin{align}
    \log \frac{1-q_i}{q_i} + \mathbb{E}_{\bm{\xi}_{\backslash i} \sim Q_{\bm{q}_{\backslash i}}} [f(i \vert \mathcal{A}_{\bm{\xi}_{\backslash i}})] = 0,
\end{align}
we obtain the update rule \eqref{eq:mean_field_update}.
We know $\mathrm{KL}(Q_{\bm{q}} \Vert P) \geq 0$, leading to the inequality $\log Z \geq L(\bm{q})$.
Therefore, we can evaluate the tightened lower bound of $\log Z$ using the optimized $\bm{q}$.

%\section{Estimating Marginal Probability of Fixed Cardinality}\label{app:rao_blackwell}

\section{Gradient of Ratio Matching}\label{app:gradient}
In this section, we derive the gradient of the loss function from ratio matching \eqref{eq:ratio_matching_dkpp}
in analytical form.
By defining
$u_{m, n} \coloneqq \exp(\tr \phi(\bm{L}[\mathcal{A}_m]) - \tr\phi(\bm{L}[\mathcal{A}^{\bar{n}}_m] ))$,
we obtain
\begin{align}
    \frac{\partial J(\bm{L})}{\partial\bm{L}}
    = \sum_{m,n} \frac{d g(u_{m,n})^2}{d u_{m,n}} \frac{\partial u_{m,n}}{\partial \bm{L}}
    \label{eq:rm_gradient_1}
    = -2\sum_{m,n} \frac{g(u_{m,n})}{(1 + u_{m,n})^2} \frac{\partial u_{m,n}}{\partial \bm{L}}.
\end{align}
Here, $\bm{U}_\mathcal{A}$ denotes the $N \times \lvert \mathcal{A} \rvert$ binary matrix
such that $\bm{L}[\mathcal{A}] = \bm{U}^\top_\mathcal{A} \bm{L} \bm{U}_\mathcal{A}$.
Then, 
\begin{align}
    \frac{\partial}{\partial \bm{L}} \tr \phi(\bm{L}[\mathcal{A}])
    = \bm{U}^\top_\mathcal{A} \phi' (\bm{L}[\mathcal{A}]) \bm{U}_\mathcal{A},
\end{align}
where $\phi'$ is the derivative of the univariate scalar function $\phi$.
Therefore, the remaining term in \eqref{eq:rm_gradient_1} becomes
\begin{align}
   \frac{\partial u_{m,n}}{\partial \bm{L}}
   = u_{m,n} (\bm{U}^\top_{\mathcal{A}_m} \phi' (\bm{L}[\mathcal{A}_m]) \bm{U}_{\mathcal{A}_m}
   - \bm{U}^\top_{\mathcal{A}^{\bar{n}}_m} \phi' (\bm{L}[\mathcal{A}^{\bar{n}}_m]) \bm{U}_{\mathcal{A}^{\bar{n}}_m}).
\end{align}
Consequently, the derivative we seek is
\begin{align}
    \label{eq:rm_gradient_L}
    \frac{\partial J(\bm{L})}{\partial\bm{L}}
    = -2\sum_{m,n} \frac{u_{m,n} g(u_{m,n})}{(1 + u_{m,n})^2}
    (\bm{U}^\top_{\mathcal{A}_m} \phi' (\bm{L}[\mathcal{A}_m]) \bm{U}_{\mathcal{A}_m}
    - \bm{U}^\top_{\mathcal{A}^{\bar{n}}_m} \phi' (\bm{L}[\mathcal{A}^{\bar{n}}_m]) \bm{U}_{\mathcal{A}^{\bar{n}}_m}).
\end{align}
For evaluating the gradient \eqref{eq:rm_gradient_L},
computing $u_{m,n}$ requires $\mathcal{O}(\lvert \mathcal{A}_m \rvert^3)$ time complexity,
and
$\bm{U}^\top_{\mathcal{A}_m} \phi' (\bm{L}[\mathcal{A}_m]) \bm{U}_{\mathcal{A}_m}$
also takes $\mathcal{O}(\lvert \mathcal{A}_m \rvert^3)$
because $\bm{U}_{\mathcal{A}_m}$ has only $\lvert \mathcal{A}_m \rvert$ non-zero elements.
Computing
$\bm{U}^\top_{\mathcal{A}^{\bar{n}}_m} \phi' (\bm{L}[\mathcal{A}^{\bar{n}}_m]) \bm{U}_{\mathcal{A}^{\bar{n}}_m}$
takes $\mathcal{O}((\lvert \mathcal{A}_m \rvert + 1)^3) =\mathcal{O}(\lvert \mathcal{A}_m \rvert^3)$.
By taking the complexity from the sum of $N \times N$ matrices into account,
we obtain the whole complexity
$\mathcal{O}(\sum_{(m,n) \in \Omega} \lvert \mathcal{A}_m \rvert^3 + \lvert \Omega \rvert N^2)
= \mathcal{O}(\lvert \Omega \rvert (\kappa^3 + N^2))$
with the minibatch $\Omega$.

In practical scenarios, $\bm{V} \in \mathbb{R}^{N \times D}$ such that $\bm{L} = \bm{V} \bm{V}^\top$
is often learned to keep $\bm{L}$ positive (semi-)definite in learning steps.
If $D < N$, the low-rank kernel matrix is obtained.
Then, the gradient with respect to $\bm{V}$ becomes
\begin{align}
    \frac{\partial J(\bm{L})}{\partial\bm{V}}
    &= 2\frac{\partial J(\bm{L})}{\partial\bm{L}} \bm{V}\\
    \label{eq:rm_gradient_V}
    &= -4\sum_{m,n} \frac{u_{m,n} g(u_{m,n})}{(1 + u_{m,n})^2}
    (\bm{U}^\top_{\mathcal{A}_m} \phi' (\bm{L}[\mathcal{A}_m]) \bm{U}_{\mathcal{A}_m} \bm{V}
    - \bm{U}^\top_{\mathcal{A}^{\bar{n}}_m} \phi' (\bm{L}[\mathcal{A}^{\bar{n}}_m]) \bm{U}_{\mathcal{A}^{\bar{n}}_m} \bm{V}).
\end{align}
Since $\bm{U}_{\mathcal{A}_m} \bm{V}$ is the $\lvert \mathcal{A}_m \rvert \times D$ dense matrix,
the time complexity of \eqref{eq:rm_gradient_V} is
$\mathcal{O}(\sum_{(m,n) \in \Omega}(\lvert \mathcal{A}_m \rvert^3 + D\lvert \mathcal{A}_m \rvert^2) + \lvert \Omega \rvert ND)
= \mathcal{O}(\lvert \Omega \rvert (\kappa^2 \max\{\kappa, D\} + ND))$.
The term $\mathcal{O}(\lvert \Omega \rvert ND)$ arises from matrix additions,
which still ensures scalability as $M$ and/or $N$ increases even if $D = N$.

%\section{Further Experiments}\label{app:experiments}

%The mean-field approximation by \eqref{eq:mean_field_update} has two hyperparameters:
%the number of iterations $T_{\mathrm{MF}}$ and the number of Monte Carlo samples for evaluating
%the expectation $M_{\mathrm{MF}}$.
%We use $T_{\mathrm{mf}} = 15$ and $M_{\mathrm{MF}} = 25$.

\section{FORMATTING INSTRUCTIONS}

To prepare a supplementary pdf file, we ask the authors to use \texttt{aistats2025.sty} as a style file and to follow the same formatting instructions as in the main paper.
The only difference is that the supplementary material must be in a \emph{single-column} format.
You can use \texttt{supplement.tex} in our starter pack as a starting point, or append the supplementary content to the main paper and split the final PDF into two separate files.

Note that reviewers are under no obligation to examine your supplementary material.

\section{MISSING PROOFS}

The supplementary materials may contain detailed proofs of the results that are missing in the main paper.

\subsection{Proof of Lemma 3}

\textit{In this section, we present the detailed proof of Lemma 3 and then [ ... ]}

\section{ADDITIONAL EXPERIMENTS}

If you have additional experimental results, you may include them in the supplementary materials.

\subsection{The Effect of Regularization Parameter}

\textit{Our algorithm depends on the regularization parameter $\lambda$. Figure 1 below illustrates the effect of this parameter on the performance of our algorithm. As we can see, [ ... ]}

\vfill

\end{document}
